# Supplementary material for: Imaging topological defects in a non-collinear antiferromagnet
Source: arXiv:2202.02243 ancillary file (2022-02-04)
Supplement: Supplementary file 1 [file supplement.pdf]

# Supplemental Material
# Imaging topological defects in a non-collinear antiferromagnet

Aurore Finco,[1] Angela Haykal,[1] Stéphane Fusil,[2] Pawan Kumar,[1]
Pauline Dufour,[2] Anne Forget,[3] Dorothée Colson,[3] Jean-Yves Chauleau,[3]
Michel Viret,[3] Nicolas Jaouen,[4] Vincent Garcia,[2] and Vincent Jacques[1]

[1]*Laboratoire Charles Coulomb, Université de Montpellier and CNRS, 34095 Montpellier, France*
[2]*Unité Mixte de Physique, CNRS, Thales, Université Paris-Saclay, 91767 Palaiseau, France*
[3]*SPEC, CEA, CNRS, Université Paris-Saclay, 91191 Gif sur Yvette, France*
[4]*Synchrotron SOLEIL, 91192 Gif-sur-Yvette, France*

## I. CALIBRATION OF THE NV-TO-SAMPLE DISTANCE

In order to determine the distance $d_{\mathrm{NV}}$ between the NV center and the sample surface, we follow the calibration procedure described in ref. [1]. First, we measure the direction of the NV center quantization axis by recording the ESR frequency as a function of the orientation of a calibrated magnetic field. We obtain the polar angle $\theta_{\mathrm{NV}} = 120°$ and the azimuthal angle $\varphi_{\mathrm{NV}} = 5°$. Then we measure a magnetic stray field profile across a well-characterized ferromagnetic stripe with perpendicular magnetic anisotropy. Using the analytical expression of the stray field generated by the edges and our knowledge of the NV center orientation, we fit the experimental profile, as shown in Fig S1, and extract the value of $d_{\mathrm{NV}} = 60 \pm 1\,\mathrm{nm}$.

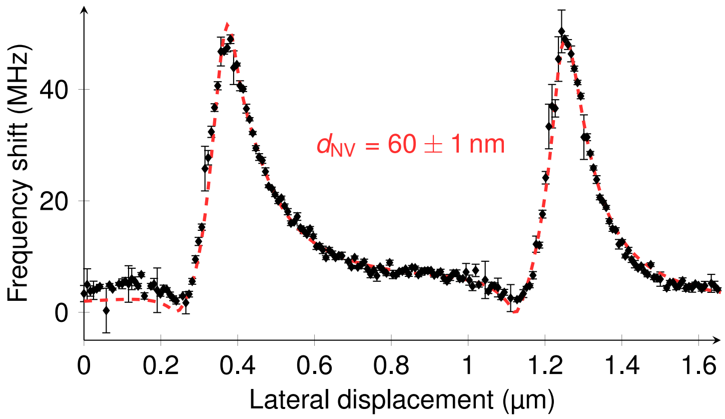


FIG. S1. Magnetic stray field profile measured across a ferromagnetic stripe, fitted analytically in order to extract the value of $d_{\mathrm{NV}}$.

## II. ANALYTICAL EXPRESSION OF THE STRAY FIELD PRODUCED BY THE $\mathbf{k_3}$ VARIANT OF THE CYCLOID

We consider a $BiFeO_3$ bulk crystal with a (001) surface, and the ferroelectric polarization $\mathbf{P}$ along the [111] direction. We want to compute the stray field $\mathbf{B}$ generated by the

magnetic texture in a domain where the cycloid is propagating along $\mathbf{k_3}$, which is parallel to the $[0\bar{1}1]$ direction. In the cyloid itself, the antiferromagnetic ordering results in a perfect compensation of the magnetic moments. Therefore, the only component of the magnetic texture contributing to the stray field is the spin density wave. We describe it as:

$$\mathbf{M}_{\mathrm{SDW}}(\mathbf{r}) = \frac{m_{\mathrm{DM}}}{a^3\sqrt{6}} \cos(\mathbf{k_3}\cdot\mathbf{r})(-2\mathbf{e}_x + \mathbf{e}_y + \mathbf{e}_z) \tag{1}$$

with $a = 3.96\,\text{Å}$ the $\mathrm{BiFeO_3}$ unit cell size. It leads to:

$$\begin{cases} M_x = -\dfrac{2m_{\mathrm{DM}}}{a^3\sqrt{6}} \cos\left(\dfrac{k}{\sqrt{2}}(y-z)\right) \\ M_y = \dfrac{m_{\mathrm{DM}}}{a^3\sqrt{6}} \cos\left(\dfrac{k}{\sqrt{2}}(y-z)\right) \\ M_z = \dfrac{m_{\mathrm{DM}}}{a^3\sqrt{6}} \cos\left(\dfrac{k}{\sqrt{2}}(y-z)\right) \end{cases} \tag{2}$$

We introduce the potential $\Phi$ such that $\mathbf{B} = -\boldsymbol{\nabla}\Phi$. This potential can be expressed as:

$$\Phi(\mathbf{r}) = -\frac{\mu_0}{4\pi}\int \mathbf{M}(\mathbf{r}')\cdot\boldsymbol{\nabla}'\frac{1}{|\mathbf{r}-\mathbf{r}'|}\mathrm{d}\mathbf{r}' \tag{3}$$

Eq.(3) is a convolution, so we can easily compute $\Phi$ in Fourier space:

$$\Phi = \mathcal{F}^{-1}\left[\mathcal{F}[\mathbf{M}]\ \mathcal{F}\left[\boldsymbol{\nabla}\left(\frac{1}{r}\right)\right]\right] \tag{4}$$

Note that we have [2]:

$$\mathcal{F}\left[\frac{1}{r}\right](q) = 2\pi\frac{e^{-|q|(z-z')}}{|q|} \quad \text{for} \quad |q|\neq 0 \quad \text{and} \quad z' < z. \tag{5}$$

For a single $\mathrm{BiFeO_3}$ layer of thickness $a$, we get:

$$\begin{aligned}\Phi = -\frac{\mu_0}{4\pi}\int_{z'=-a/2}^{z'=a/2}\Bigg(\iint_{-\infty}^{\infty}\Bigg[ & iq_x\mathcal{F}(M_x)\mathcal{F}\left(\frac{1}{r}\right) + iq_y\mathcal{F}(M_y)\mathcal{F}\left(\frac{1}{r}\right) \\ & -|q|\mathcal{F}(M_z)\mathcal{F}\left(\frac{1}{r}\right)\Bigg] e^{ixq_x+iyq_y}\,\mathrm{d}q_x\,\mathrm{d}q_y\Bigg)\,\mathrm{d}z'\end{aligned} \tag{6}$$

Rewriting Eq.(6) as $\Phi = -\frac{\mu_0}{4\pi}\int_{z'=-a/2}^{z'=a/2}(I + II + III)\,\mathrm{d}z'$, we compute each term separately.

$$\begin{aligned} I &= \iint_{-\infty}^{\infty} iq_x\mathcal{F}(M_x)\ \mathcal{F}\left(\frac{1}{r}\right)\ e^{ixq_x}e^{iyq_y}\,\mathrm{d}q_x\,\mathrm{d}q_y \\ I &= \left(\int_{-\infty}^{\infty} iq_x\delta(q_x)e^{ixq_x}\,\mathrm{d}q_x\right) \\ &\quad \times\left(\int_{-\infty}^{\infty}\frac{-2m_{\mathrm{DM}}}{a^3\sqrt{6}}\left[e^{-ikz/\sqrt{2}}\ \delta\left(\frac{k}{\sqrt{2}}-q_y\right) + e^{ikz/\sqrt{2}}\ \delta\left(\frac{k}{\sqrt{2}}+q_y\right)\right]2\pi\frac{e^{-|q|(z-z')}}{|q|})e^{iyq_y}\,\mathrm{d}q_y\right) \\ I &= 0 \end{aligned} \tag{7}$$

$$II = \iint_{-\infty}^{\infty} iq_y \mathcal{F}(M_y)\ \mathcal{F}\left(\frac{1}{r}\right)\ e^{ixq_x} e^{iyq_y}\,\mathrm{d}q_x\,\mathrm{d}q_y$$

$$II = \iint_{-\infty}^{\infty} iq_y \frac{m_{\mathrm{DM}}}{a^3\sqrt{6}}\ \frac{\delta(q_x)}{2}\left[e^{-ikz/\sqrt{2}}\ \delta\left(\frac{k}{\sqrt{2}} - q_y\right) + e^{ikz/\sqrt{2}}\ \delta\left(\frac{k}{\sqrt{2}} + q_y\right)\right] \times 2\pi \frac{e^{-|q|(z-z')}}{|q|}\ e^{ixq_x} e^{iyq_y}\,\mathrm{d}q_x\,\mathrm{d}q_y$$

$$II = -2\pi \frac{k}{\sqrt{2}} \frac{m_{\mathrm{DM}}}{a^3\sqrt{6}} \frac{e^{-k(z-z')/\sqrt{2}}}{\frac{k}{\sqrt{2}}} \frac{1}{2i}\left[e^{-ikz/\sqrt{2}} e^{iky/\sqrt{2}} - e^{ikz/\sqrt{2}} e^{-iky/\sqrt{2}}\right]$$

$$II = -2\pi \frac{m_{\mathrm{DM}}}{a^3\sqrt{6}} e^{-k(z-z')/\sqrt{2}} \sin\left(\frac{k}{\sqrt{2}}(y-z)\right) \tag{8}$$

$$III = \iint_{-\infty}^{\infty} -|q|\ \mathcal{F}(M_z)\ \mathcal{F}\left(\frac{1}{r}\right)\ e^{ixq_x} e^{iyq_y}\,\mathrm{d}q_x\,\mathrm{d}q_y$$

$$III = \iint_{-\infty}^{\infty} -|q| \frac{m_{\mathrm{DM}}}{a^3\sqrt{6}}\ \frac{\delta(q_x)}{2}\left[e^{-ikz/\sqrt{2}}\ \delta\left(\frac{k}{\sqrt{2}} - q_y\right) + e^{ikz/\sqrt{2}}\ \delta\left(\frac{k}{\sqrt{2}} + q_y\right)\right] \times 2\pi \frac{e^{-|q|(z-z')}}{|q|}\ e^{ixq_x} e^{iyq_y}\,\mathrm{d}q_x\,\mathrm{d}q_y$$

$$III = -\frac{m_{\mathrm{DM}}}{a^3\sqrt{6}} 2\pi e^{-k(z-z')} \frac{1}{2}\left[e^{-ikz/\sqrt{2}} e^{iky/\sqrt{2}} + e^{ikz/\sqrt{2}} e^{-iky/\sqrt{2}}\right]$$

$$III = -2\pi \frac{m_{\mathrm{DM}}}{a^3\sqrt{6}} e^{-k(z-z')/\sqrt{2}} \cos\left(\frac{k}{\sqrt{2}}(y-z)\right) \tag{9}$$

$$\tag{10}$$

We bring everything together and we have, still for a $BiFeO_3$ single layer:

$$\Phi = \frac{\mu_0 m_{\mathrm{DM}}}{\sqrt{3}a^3} \frac{e^{-kz/\sqrt{2}}}{k} \sinh\left(\frac{ka}{2\sqrt{2}}\right)\left[\cos\left(\frac{k}{\sqrt{2}}(y-z)\right) + \sin\left(\frac{k}{\sqrt{2}}(y-z)\right)\right] \tag{11}$$

The corresponding stray field $\mathbf{B} = -\boldsymbol{\nabla}\Phi$ is:

$$\begin{cases} B_x = 0 \\ B_y = -\dfrac{\mu_0\ m_{\mathrm{DM}}}{\sqrt{6}a^3} e^{-kz/\sqrt{2}} \sinh\left(\dfrac{ka}{2\sqrt{2}}\right)\left[\cos\left(\dfrac{k}{\sqrt{2}}(y-z)\right) - \sin\left(\dfrac{k}{\sqrt{2}}(y-z)\right)\right] \\ B_z = \sqrt{\dfrac{2}{3}} \dfrac{\mu_0\ m_{\mathrm{DM}}}{a^3} e^{-kz/\sqrt{2}} \sinh\left(\dfrac{ka}{2\sqrt{2}}\right) \cos\left(\dfrac{k}{\sqrt{2}}(y-z)\right) \end{cases} \tag{12}$$

To get the value of the stray field for the whole crystal of thickness $t$ constituted of $N = \frac{t}{a}$ layers, we have to sum these terms with $z \to z + ja$ ($j \in [0, N-1]$). Defining:

$$\mathcal{S} = \sum_{j=0}^{N-1} e^{-k(z+ja)/\sqrt{2}} e^{\frac{ik}{\sqrt{2}}(y-z+ja)} = e^{-kz/\sqrt{2}} e^{ik(y-z)/\sqrt{2}}\ \frac{1 - e^{-kt(1+i)/\sqrt{2}}}{1 - e^{-ka(1+i)/\sqrt{2}}} \tag{13}$$

and

$$\mathcal{A} = \frac{\mu_0 m_{\rm DM}}{\sqrt{3}a^3}\sinh\left(\frac{ka}{2\sqrt{2}}\right) \tag{14}$$

we reach the final expression for the stray field generated by the spin density wave in a domain where the cycloid propagates along $\mathbf{k_3}$ in a $BiFeO_3$ crystal of thickness $t$:

$$\begin{cases} B_x = 0 \\ B_y = -\frac{\mathcal{A}}{\sqrt{2}}\left(\mathrm{Re}\{\mathcal{S}\} - \mathrm{Im}\{\mathcal{S}\}\right) \\ B_z = \sqrt{2}\mathcal{A}\,\mathrm{Re}\{\mathcal{S}\} \end{cases} \tag{15}$$

## III. WAVEVECTOR ELLIPSE

If we assume that the wavevector $\mathbf{k}$ of the cycloid rotates but stays in the (111) plane and that the period $\lambda_b$ of the cycloid does not depend on the direction of $\mathbf{k}$, the ensemble of all the possible cycloid wavevectors describes a circle in the (111) plane. Both with NV magnetometry and REXS, we probe the surface plane, which is a (001) plane of the bulk $BiFeO_3$ crystal. The projection of the circle of radius $k = \frac{2\pi}{\lambda_b}$ in (111) plane onto the (001) is the ellipse depicted in Fig. S2. Its polar equation, with $\theta = 0°$ aligned along $\mathbf{k_1}$ is:

$$r(\theta) = \frac{2\pi}{\lambda_b}\frac{1}{\sqrt{3 - 2\cos^2\theta}} \tag{16}$$

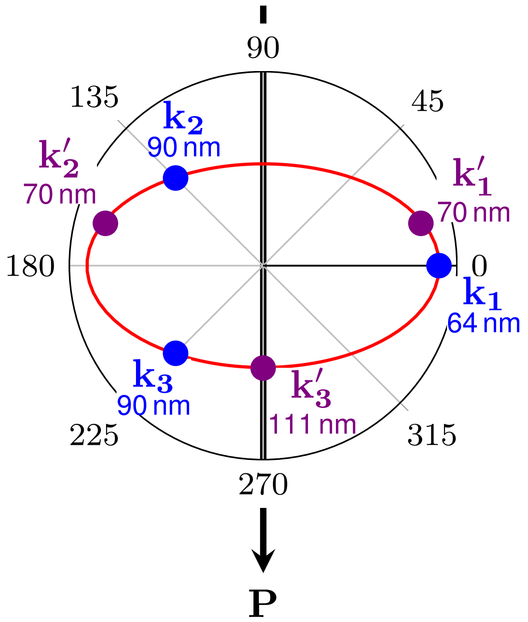


FIG. S2. Sketch of the ellipse corresponding to the projection on the (001) plane of a circle of radius $k = \frac{2\pi}{\lambda_b}$ in the (111) plane. The propagation directions corresponding to the cycloid type I ($\mathbf{k_1}$, $\mathbf{k_2}$ and $\mathbf{k_3}$) and to the cycloid type II ($\mathbf{k'_1}$, $\mathbf{k'_2}$ and $\mathbf{k'_3}$) are indicated, as well as the corresponding projected period.

---

[1] T. Hingant, J.-P. Tetienne, L. J. Martínez, K. Garcia, D. Ravelosona, J.-F. Roch, and V. Jacques, Phys. Rev. Applied **4**, 014003 (2015).

[2] R. J. Blakely, *Potential theory in gravity and magnetic applications* (Cambridge University Press, 1995).
